# Supplementary material for: Efficient Facial Landmark Detection for Embedded Systems
Source: arXiv:2407.10228 source file (2024-07-14)
Supplement: Supplementary file 1 [file X_supp.tex]

\clearpage
\setcounter{page}{1}

\section{Supplementary Material}
\label{sec:additionalqualitativeresults}

\subsection{Visualize TFLlite Model}
\cref{fig:visualize-tflite} shows the detail architecture of our model, if the figure is too small, you may visualize yourself by using the following tool: https://netron.app/

Our model compose of of four EffBlocks,
The configuration of each EffBlock is set as

\begin{itemize}
\item 1. A conventional convolutional layer with 8 filters and a VoVNet with 2 conventional convolutional layers, whose feature dimension is 4.
\item 2. A depthwise seperable convolutional layer with 8 filters and a VoVNet with 3 conventional convolutional layers, whose feature dimension is 8.
\item 3. A depthwise seperable convolutional layer with 16 filters and a VoVNet with 3 conventional convolutional layers, whose feature dimension is 16.
\item 4. A depthwise seperable convolutional layer with 32 filters and a VoVNet with 3 conventional convolutional layers, whose feature dimension is 16.
\end{itemize}

The decoder decodes the feature map into a 256-dimensional feature vector. The detection head consists of three linear blocks with 32 units each, followed by concatenation. Finally, a linear layer is used to predict the position of facial landmarks.

\begin{figure}[t]
    \centering
    \includegraphics[width=0.2\columnwidth]{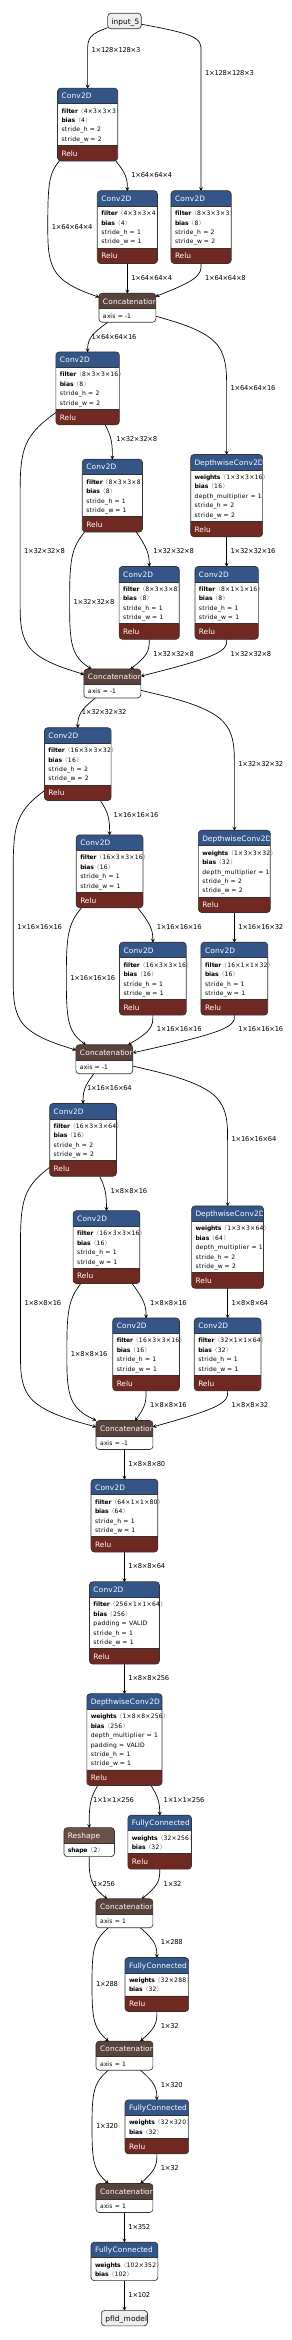}
    \vspace{-0.5cm}
    \caption{Visualization of tflite model}
    \vspace{-0.2cm}
    \label{fig:visualize-tflite}
\end{figure}
